# Supplementary material for: A Unique Crystal Structure of Ca$_2$RuO$_4$ in the Current Stabilized Semi-Metallic State
Source: arXiv:1806.06455 ancillary file (2019-05-21)
Supplement: Supplementary file 1 [file supplemental.pdf]

# Supplemental Material: A Unique Crystal Structure of $Ca_2RuO_4$ in the Current Stabilized Semi-Metallic State

J. Bertinshaw,[1] N. Gurung,[1] P. Jorba,[2] H. Liu,[1] M. Schmid,[3,4,1] D. T. Mantadakis,[1] M. Daghofer,[3,4] M. Krautloher,[1] A. Jain,[1] G. H. Ryu,[1] O. Fabelo,[5] P. Hansmann,[6,1] G. Khaliullin,[1] C. Pfleiderer,[2] B. Keimer,[1] and B. J. Kim[1,7,8]

[1]*Max Planck Institute for Solid State Research, Heisenbergstraße 1, D-70569 Stuttgart, Germany*

[2]*Physik-Department, Technische Universität München, D-85748 Garching, Germany*

[3]*Institute for Functional Matter and Quantum Technologies, University of Stuttgart, Pfaffenwaldring 57, D-70550 Stuttgart, Germany*

[4]*Center for Integrated Quantum Science and Technology, University of Stuttgart, Pfaffenwaldring 57, D-70550 Stuttgart, Germany*

[5]*Institut Laue Langevin, BP 156, F-38042 Grenoble cedex 9, France*

[6]*Max Planck Institute for Chemical Physics of Solids, Nöthnitzerstr Straße 40, D-01187 Dresden, Germany*

[7]*Department of Physics, Pohang University of Science and Technology, Pohang 790-784, South Korea*

[8]*Center for Artificial Low Dimensional Electronic Systems, Institute for Basic Science (IBS), 77 Cheongam-Ro, Pohang 790-784, South Korea*

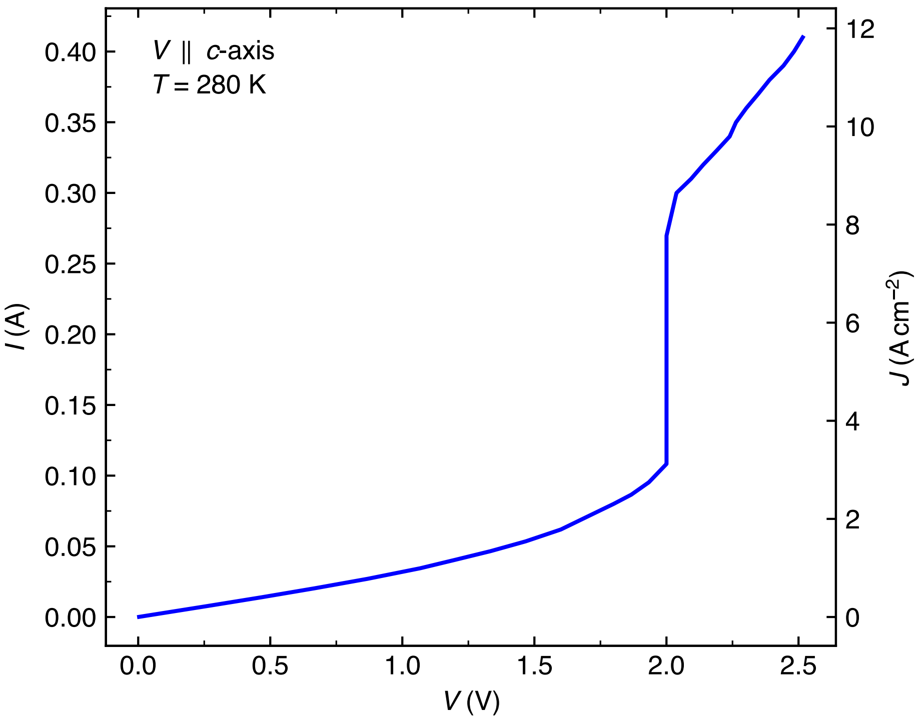


Figure S1. Voltage-current curve obtained *in-situ* while conducting the single crystal neutron diffraction study. Measurements were made using a two-probe method with the voltage applied parallel to the $c$-axis at $T = 280\,\mathrm{K}$. The dimensions of the crystal used in this study were approximately $3.5\,\mathrm{mm}^2 \times 0.4\,\mathrm{mm}$.

Table SI. Neutron diffraction structural least-squares refinement in the orthorhombic *Pbca* space group at $T = 130\,\mathrm{K}$ of the equilibrium S-phase and non-equilibrium S*- and L*-phases at $J = 10\,\mathrm{A\,cm^{-2}}$. Bond lengths and the $RuO_6$ distortions derived from the atomic positions presented here are shown in Table 1 of the main text.

| Phase | S-phase | S*-phase | L*-phase |
|---|---|---|---|
| Temperature | 130 | 130 | 130 |
| Space group | *Pbca* | *Pbca* | *Pbca* |
| $a$ (Å) | 5.3842(8) | 5.404(4) | 5.341(5) |
| $b$ (Å) | 5.6158(9) | 5.547(4) | 5.436(6) |
| $c$ (Å) | 11.7461(11) | 11.848(8) | 12.153(9) |
| Ca $x$ | 0.0034(4) | 0.0059(6) | 0.0076(7) |
| Ca $y$ | 0.0591(4) | 0.0518(9) | 0.0481(11) |
| Ca $z$ | 0.3524(1) | 0.3524(4) | 0.3509(4) |
| O(1) $x$ | 0.1949(3) | 0.1957(6) | 0.1954(7) |
| O(1) $y$ | 0.3010(4) | 0.3009(7) | 0.3020(8) |
| O(1) $z$ | 0.0277(2) | 0.0264(4) | 0.0216(4) |
| O(2) $x$ | -0.0695(2) | -0.0650(6) | -0.0613(8) |
| O(2) $y$ | -0.0216(2) | -0.0184(8) | -0.0189(9) |
| O(2) $z$ | 0.1642(1) | 0.1642(3) | 0.1639(4) |
| Rf-factor | 3.11 | 4.24 | 4.96 |

## DMFT CALCULATION DETAILS

In the following we provide additional technical details and plots of the k-resolved single particle spectra. Our calculations were performed in the framework of density-functional theory (DFT) in its local density approximation (LDA) + dynamical mean-field theory (DMFT). Spin-orbit coupling (SOC) is included in our calculations as $t_{2g}$-projection of $\zeta \sum_i^{N_e} \mathbf{l}_i \mathbf{s}_i$, where we sum over all $N_e$ electrons and approximate $\zeta$ by its Hartree-Fock value of $\zeta = 0.16\,\mathrm{eV}$ [1]. For the DMFT self-consistency we use a continuous-time quantum Monte Carlo impurity solver in the hybridization expansion (published as part of the TRIQS library[2, 3]). Electronic interaction is approximated by the (SU(2) symmetric) Kanamori operator with (previously established [4–6]) values for the parameters $U = 1.9\,\mathrm{eV}$ and $J_H = 0.4\,\mathrm{eV}$ for all structures.

### Effective model and orbital occupations in DMFT

The effective three band model for the DMFT calculations was derived by projecting the LDA Kohn-Sham states to a Wannier basis [7, 8] in a low energy window of the range $[-2,\ 1]\,\mathrm{eV}$ around the Fermi level $E_F = 0$. Bands at these energies are dominantly Ru $4d - t_{2g}$-states. Note that the "$t_{2g}$" label is strictly precise only in cubic symmetry. All considered structures, however, are lower in symmetry: we find sizable tetragonal splittings of $E_{\mathrm{xy}} \neq E_{\mathrm{xz/yz}}$ plus small orthorhombic distortions leading to an additional split $E_{\mathrm{xz}} \neq E_{\mathrm{yz}}$. The derived models reveal a clear trend on the single particle level: The tetragonal crystal-field splitting of $xy$ and $xz/yz$ orbitals decreases when a current drives the low temperature equilibrium S-phase $E_{\mathrm{xz/yz}} - E_{\mathrm{xy}} = 0.32\,\mathrm{eV}$ to $0.29\,\mathrm{eV}$ for the non-equilibrium S*-phase and $0.19\,\mathrm{eV}$ for the L*-phase (the $T = 400\,\mathrm{K}$ high temperature phase shows the smallest tetragonal splitting of all structures with merely $0.1\,\mathrm{eV}$). The orthorhombic distortions are all at least one order of magnitude smaller $\mathcal{O}\,(10^{-2}\,\mathrm{eV})$. The DMFT results show that this materials trend remains visible in the orbital occupations of the correlated ground state reported in Table SII.

As one might expect, the similar crystal structures lead to similar orbital occupation numbers. The S-phase has the largest tetragonal splitting between $xy$ and $xz/yz$ states and the largest orbital polarization with fillings of $n_{xz} = 1.11$, $n_{yz} = 1.13$, and $n_{xy} =$

Table SII. Occupation numbers of three $t_{2g}$ orbitals from DMFT calculations. The structural similarity is reflected by similar occupation numbers between the S- and S*-phases, and between the L*- and 400 K phases.

| | S | S* | L* | $T = 400\,\mathrm{K}$ |
|---|---|---|---|---|
| $n_{\mathrm{xz}}$ | 1.11 | 1.16 | 1.28 | 1.34 |
| $n_{\mathrm{yz}}$ | 1.13 | 1.14 | 1.25 | 1.32 |
| $n_{\mathrm{xy}}$ | 1.76 | 1.70 | 1.47 | 1.34 |
| $n_{\mathrm{tot}}$ | 4.00 | 4.00 | 4.00 | 4.00 |

1.76 (these numbers show further that the orthorhombic distortions are indeed not very pronounced). Irrespective of a qualitative change in the metallicity, the S*-phase has very similar occupations, as shown in Table SII. Also, the structural similarity of the L*- and 400 K phases is reflected in similar orbital fillings.

### DMFT Single Particle Spectra

Supplementary to Fig. 3 in the main text, here we provide additional plots of $A(\omega, \mathbf{k})$ and $A(\omega)$ over a larger energy range [-3, 1] eV in Figs. S2, S3, S4 and S5. The four panels in each figure show orbitally resolved (a) - (c) and total (d) spectra.

Fig. S2 shows spectra for the 130 K S-phase, which are insulating with a fully developed gap of $\sim 0.2\,\mathrm{eV}$. The gap is formed between a $xy$-dominated lower-Hubbard band (roughly centered around $-1.5\,\mathrm{eV}$) and a $xz/yz$-dominated upper-Hubbard band ($\approx 0.5\,\mathrm{eV}$). Even though spin-orbit effects mix $xz$, $xz$, and $xy$ states to some extent, their contribution to the spectral features can be distinguished reasonably well. The agreement of our calculations with experimental ARPES data [9, 10] is very satisfactory: We find a wide dispersive band of $xy$ character at energies centered around $-2.0\,\mathrm{eV}$ which is the same value as seen in experiment. Further $xy$ weight is located at around $-0.3\,\mathrm{eV}$ which is slightly closer to the Fermi level than the experimental value of $-0.5\,\mathrm{eV}$. The $xz/yz$ spectral weight, on the other hand, is mostly distributed in a non-dispersive and incoherent broad band spanning from $-2.0\,\mathrm{eV}$ to $-1.0\,\mathrm{eV}$ which is again in excellent agreement with the experimental results.

Additionally a small $xz/yz$ contribution to the spectrum around $-0.3\,\text{eV}$ is found which originates from the SOC mixture with the $xy$ excitations at the same energy.

Driving the S-phase to the S*-phase leads to a redistribution of spectral weight from the Hubbard bands towards the Fermi level. This transfer is sufficient to close the insulating gap of the S-phase and to create a semi-metallic state as shown in Fig. S3. Most of the spectral weight around the Fermi level originates from quasi-particle bands crossing $E_F$ between $\Gamma$ and $X/Y$. The hole pockets is derived mostly from $xy$ bands, while $xz/yz$ orbitals dominate the electron pockets; however, this assignment is only qualitative since spin-orbit coupling and low-symmetry distortions tend to mix the orbitals. The structure of the high-energy Hubbard bands remains very similar to the equilibrium S-phase.

Larger currents stabilize the L*-phase with even smaller tetragonal distortions and larger transfer of spectral weight to the Fermi level than in the S*-phase. The similarity of the crystal structure in L*- and 400 K phase is reflected also in their correlated but metallic single particle spectra as seen in Fig. S4 and Fig. S5.

Overall, the LDA+DMFT single particle spectra illustrate the extreme sensitivity of the electronic structure to the minor structural changes in the current induced state. We also note the absence of a full orbital polarization, and contributions of all three orbitals are present both in the Hubbard bands as well as in quasiparticle bands around $E_F$.

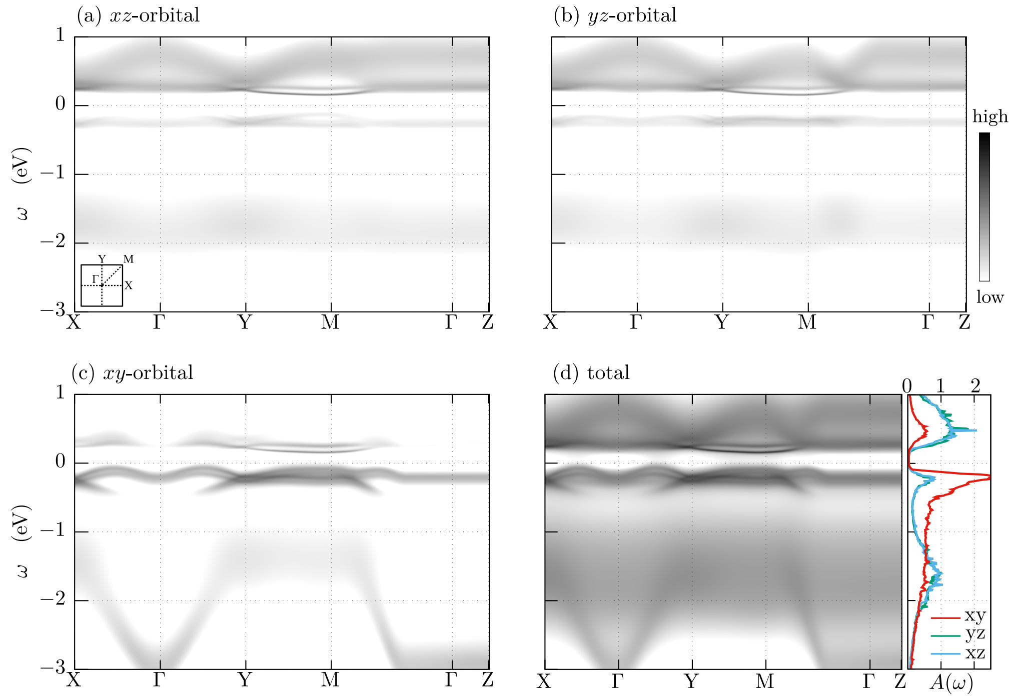


Figure S2. $T = 130\,\mathrm{K}$ equilibrium S-phase: DMFT intensity map of the single particle spectral function $A(\omega, \mathbf{k})$ (in arbitrary units, dark color implies high intensity) as a function of energy $\omega$ and momentum $\mathbf{k}$ along high-symmetry directions in the orthorhombic Brillouin zone, projected on the (a) $xz$-orbital, (b) $yz$-orbital and (c) $xy$-orbital. Panel (d) shows the total spectral function $A(\omega, \mathbf{k})$ (left) and orbital resolved local spectra $A(\omega)$ (right, in units of 1/eV).

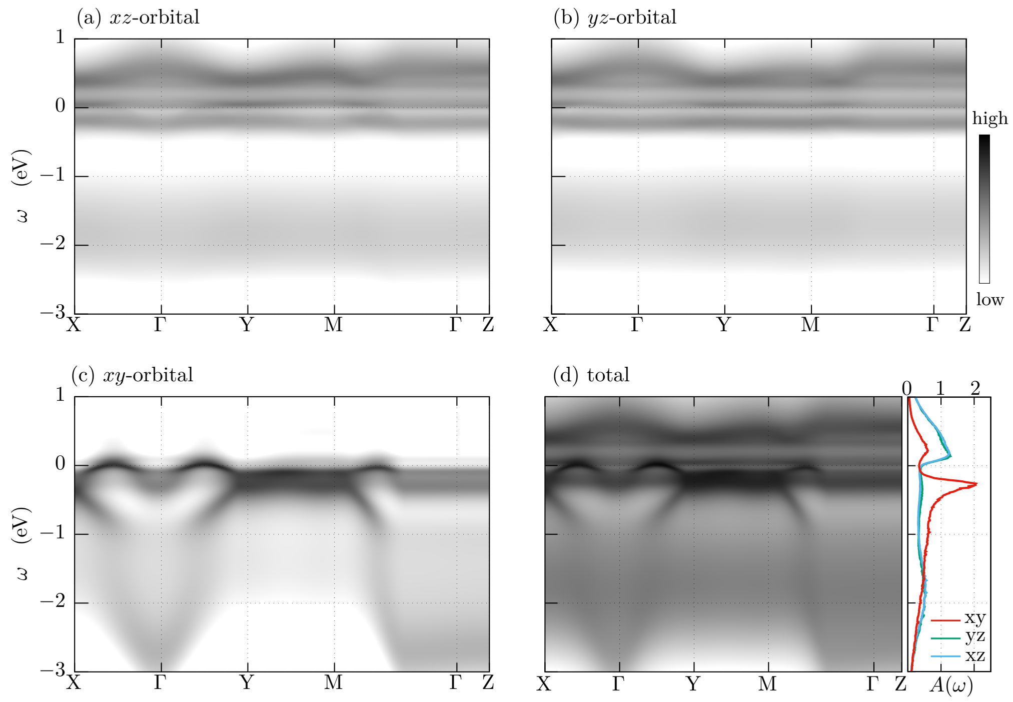


Figure S3. Non-equilibrium S*-phase: DMFT intensity map of the single particle spectral function $A(\omega, \mathbf{k})$ (in arbitrary units, dark color implies high intensity) as a function of energy $\omega$ and momentum $\mathbf{k}$ along high-symmetry directions in the orthorhombic Brillouin zone, projected on the (a) $xz$-orbital, (b) $yz$-orbital and (c) $xy$-orbital. Panel (d) shows the total spectral function $A(\omega, \mathbf{k})$ (left) and orbital resolved local spectra $A(\omega)$ (right, in units of 1/eV).

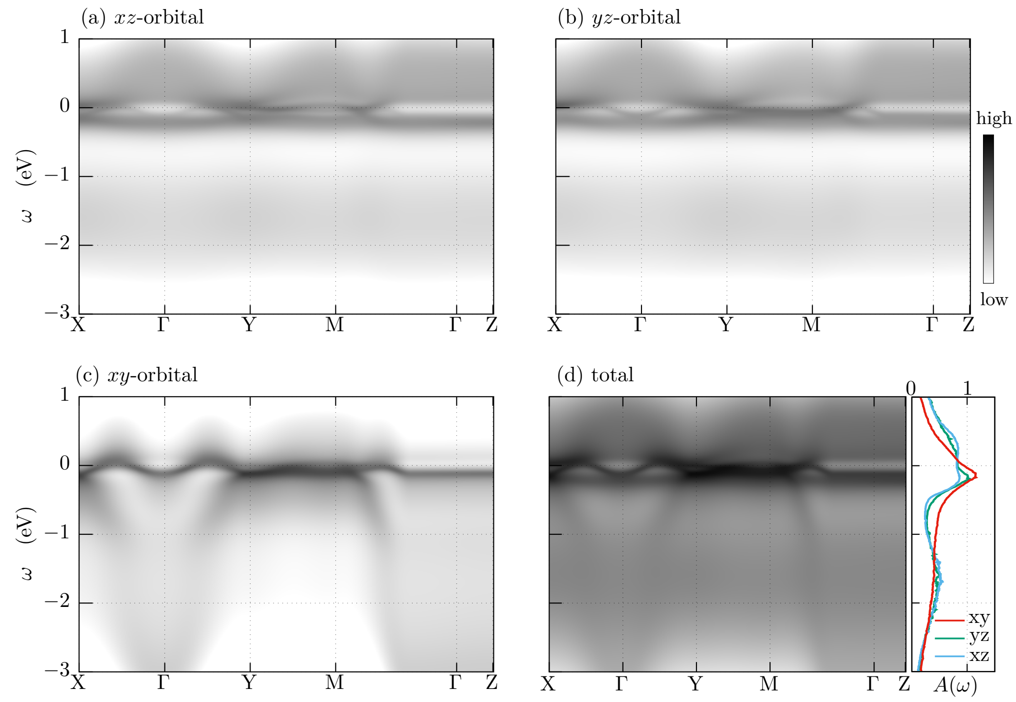


Figure S4. Non-equilibrium L*-phase: DMFT intensity map of the single particle spectral function $A(\omega, \mathbf{k})$ (in arbitrary units, dark color implies high intensity) as a function of energy $\omega$ and momentum $\mathbf{k}$ along high-symmetry directions in the orthorhombic Brillouin zone, projected on the (a) $xz$-orbital, (b) $yz$-orbital and (c) $xy$-orbital. Panel (d) shows the total spectral function $A(\omega, \mathbf{k})$ (left) and orbital resolved local spectra $A(\omega)$ (right, in units of 1/eV).

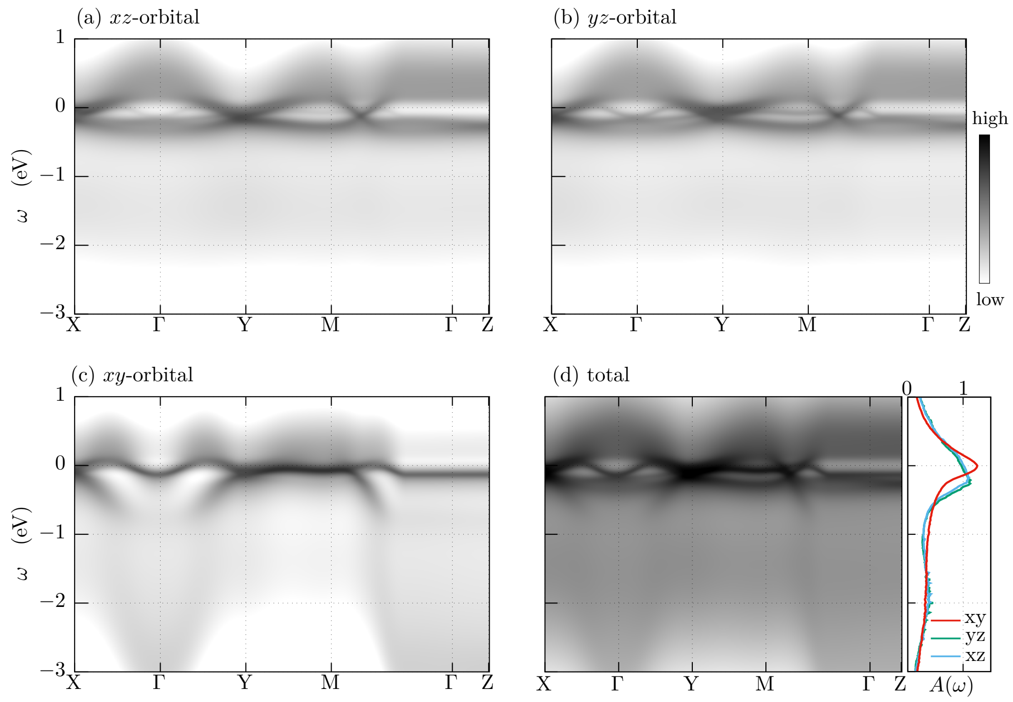


Figure S5. $T = 400\,\mathrm{K}$ equilibrium phase: DMFT intensity map of the single particle spectral function $A(\omega, \mathbf{k})$ (in arbitrary units, dark color implies high intensity) as a function of energy $\omega$ and momentum $\mathbf{k}$ along high-symmetry directions in the orthorhombic Brillouin zone, projected on the (a) $xz$-orbital, (b) $yz$-orbital and (c) $xy$-orbital. Panel (d) shows the total spectral function $A(\omega, \mathbf{k})$ (left) and orbital resolved local spectra $A(\omega)$ (right, in units of 1/eV).

## DFT+$U$ CALCULATION DETAILS

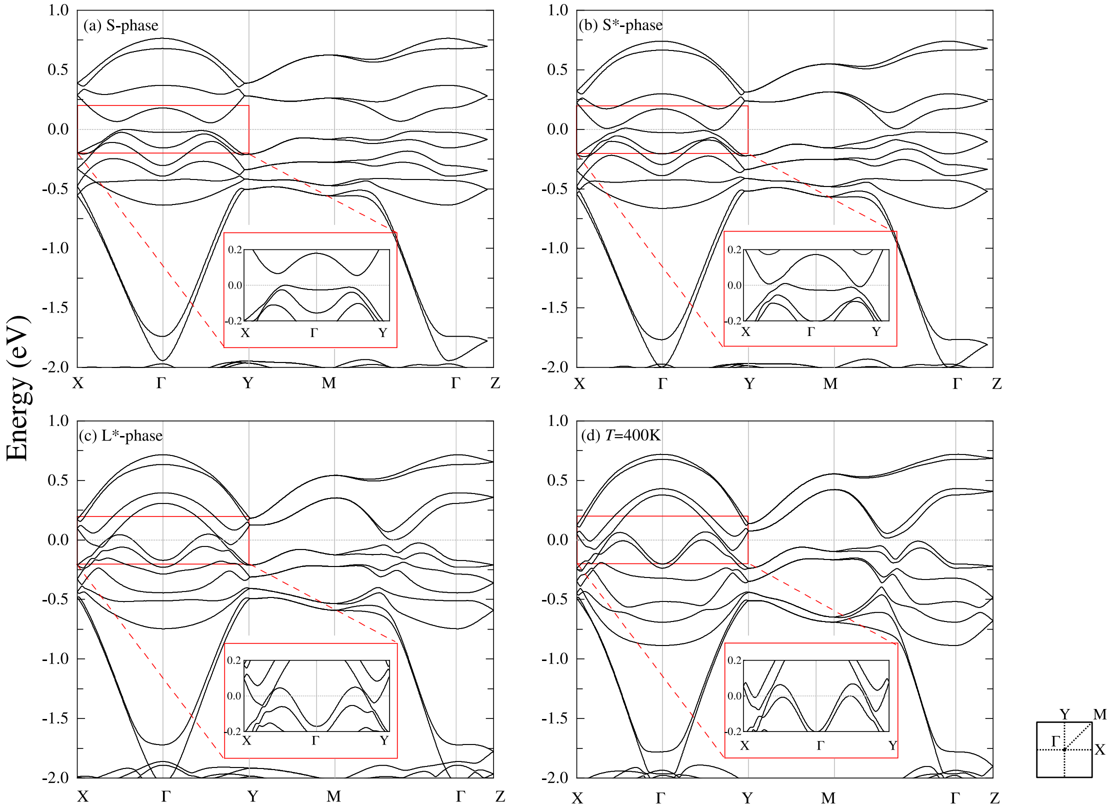


Figure S6. DFT+U band structure calculations based on the $T = 130$ K structures of the (a) equilibrium S-phase, non-equilibrium (b) S*- and (c) L*-phases, and on the (d) $T = 400$ K structure. The insets plot the region along $X$-$\Gamma$-$Y$ close to the Fermi level. The insulating gap in S-phase (a) is closed in the non-equilibrium phases (b) and (c), revealing the formation of electron and hole pockets and indicating semi-metallic behavior.

Using experimental lattice structures, nonmagnetic electronic structure calculation were carried out using the WIEN2K code [11] with a full potential linearized augmented planewave method and together with the Perdew/Burke/Ernzerhof parameterization of the generalized gradient approximation as exchange-correlation functional. The basis functions were expanded to $R_{mt}K_{\max} = 7$ (where $R_{mt}$ is the smallest of the muffin-tin sphere radii and $K_{\max}$ is the largest reciprocal lattice vector used in the plane-wave expansion) and the Brillouin zone was sampled by 10,000 k points. The SOC interaction was included through the second-order variational procedure [12]. The local Coulomb repulsion [13] parameter for Ru

orbitals was set to $U_{\text{eff}} = 2.0\,\text{eV}$ during the calculations.

The Ru-ion $t_{2g}$ orbitals represent the main contribution to the region around the Fermi level for all structures, with some admixture of O $2p$ bands due to hybridization effects; the unoccupied $e_g$ bands (not shown) are located ∼1 eV above the $t_{2g}$ band.

Even though the DFT+U method misses local correlations and associated Hubbard bands, it gives the results qualitatively consistent with our observations. Namely, there is an insulating band gap near the Fermi level in the equilibrium S-phase, while the bands slightly overlap in the non-equilibrium phases, resulting in semi-metallic state with small electron and hole pockets. This is due to an increase of the bandwidth, caused by the current-induced structural changes. The reduced $RuO_6$ distortions (hence the reduced orbital disproportionation) in the non-equilibrium phases work in favor of metallic solution. We also note that at the low-energies near the Fermi level, evolution of DFT+U band dispersions show the trends qualitatively similar to our DMFT calculations, see Fig. 3 in the main text.


[1] A. Abragam and B. Bleaney, *Electron Paramagnetic Resonance of Transition Ions*, The International Series of Monographs on Physics (Clarendon P, Oxford, 1970).

[2] O. Parcollet, M. Ferrero, T. Ayral, H. Hafermann, I. Krivenko, L. Messio, and P. Seth, Comput. Phys. Commun. **196**, 398 (2015).

[3] P. Seth, I. Krivenko, M. Ferrero, and O. Parcollet, Comput. Phys. Commun. **200**, 274 (2016).

[4] J. Kanamori, Prog. Theor. Phys. **30**, 275 (1963).

[5] M. Kim, J. Mravlje, M. Ferrero, O. Parcollet, and A. Georges, Phys. Rev. Lett. **120**, 126401 (2018).

[6] J. Mravlje, M. Aichhorn, T. Miyake, K. Haule, G. Kotliar, and A. Georges, Phys. Rev. Lett. **106**, 096401 (2011).

[7] G. Kresse and J. Furthmüller, Phys. Rev. B **54**, 11169 (1996).

[8] A. A. Mostofi, J. R. Yates, G. Pizzi, Y.-S. Lee, I. Souza, D. Vanderbilt, and N. Marzari, Comput. Phys. Commun. **185**, 2309 (2014).

[9] D. Sutter, C. G. Fatuzzo, S. Moser, M. Kim, R. Fittipaldi, A. Vecchione, V. Granata, Y. Sassa, F. Cossalter, G. Gatti, M. Grioni, H. M. Rønnow, N. C. Plumb, C. E. Matt, M. Shi, M. Hoesch,

T. K. Kim, T.-R. Chang, H.-T. Jeng, C. Jozwiak, A. Bostwick, E. Rotenberg, A. Georges, T. Neupert, and J. Chang, Nat. Commun. **8**, 15176 (2017).

[10] S. Riccò, M. Kim, A. Tamai, S. McKeown Walker, F. Y. Bruno, I. Cucchi, E. Cappelli, C. Besnard, T. K. Kim, P. Dudin, M. Hoesch, M. J. Gutmann, A. Georges, R. S. Perry, and F. Baumberger, Nat. Commun. **9**, 4535 (2018).

[11] P. Blaha, K. Schwarz, G. K. H. Masden, D. Kvasnicka, and J. Luitz, *WIEN2k, An Augmented Plane Wave + Local Orbitals Program for Calculating Crystal Properties* (Karlheinz Schwarz, Techn. Universität Wien, Austria, Wein, Austria, 2001).

[12] D. D. Koelling and B. N. Harmon, J. Phys. C Solid State Phys. **10**, 3107 (1977).

[13] V. I. Anisimov, F. Aryasetiawan, and A. I. Lichtenstein, J. Phys. Condens. Matter **9**, 767 (1997).
